# Supplementary material for: Highlighting Named Entities in Input for Auto-Formulation of Optimization Problems
Source: arXiv:2212.13201 source file (2023-12-12)
Supplement: Supplementary file 1 [file appendix.tex]

% \appendix
% \section*{Appendix}
% \section{Noisy Named Entities}
% \label{appendix:noisy_named_entities}
% To add noise to named entities in the NL4Opt Generation dataset, each span is modified with a probability of $p$. With an equal mix, we either drop the span completely, mislabel it or change its start and end positions. We ensure that no two spans overlap. For our experiments, two datasets with noisy named entities are generated for $p = 0.2$ and $p = 0.5$. To quantify the extent of the noise in the named entity tags, we use the micro-averaged F1 score to compare the named entities in the generated and original datasets. Table \ref{tab:noise_f1} shows these scores, and Figure \ref{fig:noisy_ne_example} shows an example from the noisy datasets.

% \begin{table}[t]
%     \centering
%     \caption{Comparison of noisy named entities with the original ground-truth labels (micro-averaged F1).}
%     \label{tab:noise_f1}
%     \begin{small}
%     \begin{sc}
%     \setlength{\tabcolsep}{5pt}
%     \begin{tabular}{llll}
%     \toprule
%     $p$ & Train & Dev & Test \\
%     \midrule
%     0.2 & 0.8333 & 0.8397 & 0.8353 \\
%     0.5 & 0.5783 & 0.5742 & 0.5822 \\
%     \bottomrule
%     \end{tabular}
%     \end{sc}
%     \end{small}
% \end{table}

% \begin{figure}[t]
%     \centering
%     \begin{tikzpicture}[font=\scriptsize\sffamily]
%     \node [text width=0.98\textwidth] {A berry picker must pick \colorbox{CONSTDIR}{\strut {\tiny \textsc{const\_dir}} at least} \colorbox{LIMIT}{\strut {\tiny \textsc{limit}} 3000} strawberries and \colorbox{LIMIT}{\strut {\tiny \textsc{limit}} 15000} raspberries. He visits two farms. For each hour at \colorbox{VAR}{\strut {\tiny \textsc{var}} farm 1} he spends, \colorbox{PARAM}{\strut {\tiny \textsc{param}} he can} pick \colorbox{PARAM}{\strut {\tiny \textsc{param}} 50} strawberries and \colorbox{PARAM}{\strut {\tiny \textsc{param}} 300} raspberries. For each hour at farm 2 he spends, he can catch 70 strawberries and \colorbox{PARAM}{\strut {\tiny \textsc{param}} 200} raspberries. How many \colorbox{OBJDIR}{\strut {\tiny \textsc{obj\_dir}} hours} should he spend at each farm to \colorbox{OBJDIR}{\strut {\tiny \textsc{obj\_dir}} minimize} the \colorbox{OBJNAME}{\strut {\tiny \textsc{obj\_name}} amount of time} he spends at both farms?};
%     \end{tikzpicture}
%     \caption{An example of the input from the noisy dataset generated using $p = 0.5$. See Fig.~\ref{fig:overview} for the ground truth named entity spans and their labels.}
%     \label{fig:noisy_ne_example}
% \end{figure}
